# Supplementary material for: The Hitchin index in cohomogeneity one nearly K\"ahler structures
Source: arXiv:2410.21106 source file (2024-12-10)
Supplement: Supplementary file 1 [file SC.tex]

\documentclass[main.tex]{subfiles}
\begin{document}
\section{Taylor expansions}
\label{appendix}
\section{The cohomogeneity one case}
\subsection{Differential forms one the sine cone}
Consider a closed Riemannian manifold $(\Sigma^n, g)$ and its corresponding sine cone $M = (\Sigma \times [0, \pi], dt^2 + \sin^2(t) g_{\Sigma})$. We a Laplacian $d + d^*$ acting on 2-forms. Here we collect some useful explicit formulas. It is useful to decompose the exterior differential between the $\Sigma$ component and the temporal direction. For a $k$-form $\gamma$, we write:
\[
d\alpha = d_{\Sigma} + (-1)^k dt \wedge \frac{\partial \alpha}{\partial t}.
\]

The Hodge star on the sine cone and on $\Sigma$ are related by the following identities: For $\alpha \in [TODO]$
\[
* (dt \wedge \alpha) = s^{(n+1) - 2k} *_{\Sigma} \alpha, \quad * \beta = (-1)^k s^{(n-1) - 2k} dt \wedge *_{\Sigma} \beta.
\]

A direct computation yields the following lemma:

\textbf{Lemma A.1.} Let $\eta = s^{\lambda}(s^{k-1} dt \wedge \alpha + s^k \beta)$ be a $k$-form on the sine cone. We get:
\[
* \eta = s^{\lambda + n - k} *_{\Sigma} \alpha + (-1)^k s^{\lambda + n - 1 - k} dt \wedge *_{\Sigma} \beta,
\]
\[
d\eta = s^{\lambda + k - 1} dt \wedge \left[(\lambda + k) c \beta - d_{\Sigma} \alpha + (-1)^k s \frac{\partial \beta}{\partial t}\right] + s^{\lambda + k} d_{\Sigma} \beta,
\]
\[
d^* \eta = s^{\lambda + k - 2} \left[d^*_{\Sigma} \beta - (\lambda + n - k) c \alpha + (-1)^k s \frac{\partial \alpha}{\partial t}\right] - s^{\lambda + k - 3} dt \wedge d^*_{\Sigma} \alpha.
\]

\[
\Delta \eta = s^{\lambda + k - 3} dr \wedge \left[ \Delta \alpha - (\lambda + n - k) \left[(\lambda + k - 2) + (\lambda + k - 1) s^2\right] \alpha - 2c d^*_{\Sigma} \beta - (2\lambda + n - 1) sc \frac{\partial \alpha}{\partial t} - s^2 \frac{\partial^2 \alpha}{\partial t^2} \right]
\]
\[
+ s^{\lambda + k - 2} \left[ \Delta \beta - (\lambda + k) \left[(\lambda + n - k - 2) + (\lambda + n - k - 1) s^2\right] \beta - 2c d_{\Sigma} \alpha - (2\lambda + n - 1) sc \frac{\partial \beta}{\partial t} - s^2 \frac{\partial^2 \beta}{\partial t^2} \right].
\]
